# Supplementary material for: UFO: A unified method for controlling Understandability and Faithfulness Objectives in concept-based explanations for CNNs
Source: arXiv:2303.15632 source file (2023-03-27)
Supplement: Supplementary file 1 [file remainder_group_supp.tex]

\begin{figure*}[t]
    \centering
    \begin{tabular}{c|c|c}
    \toprule
    & shopping-dining (display counters?) & home-hotel (?) \\\midrule
sf, mu & \raisebox{-0.4\totalheight}{\includegraphics[width=0.4\textwidth]{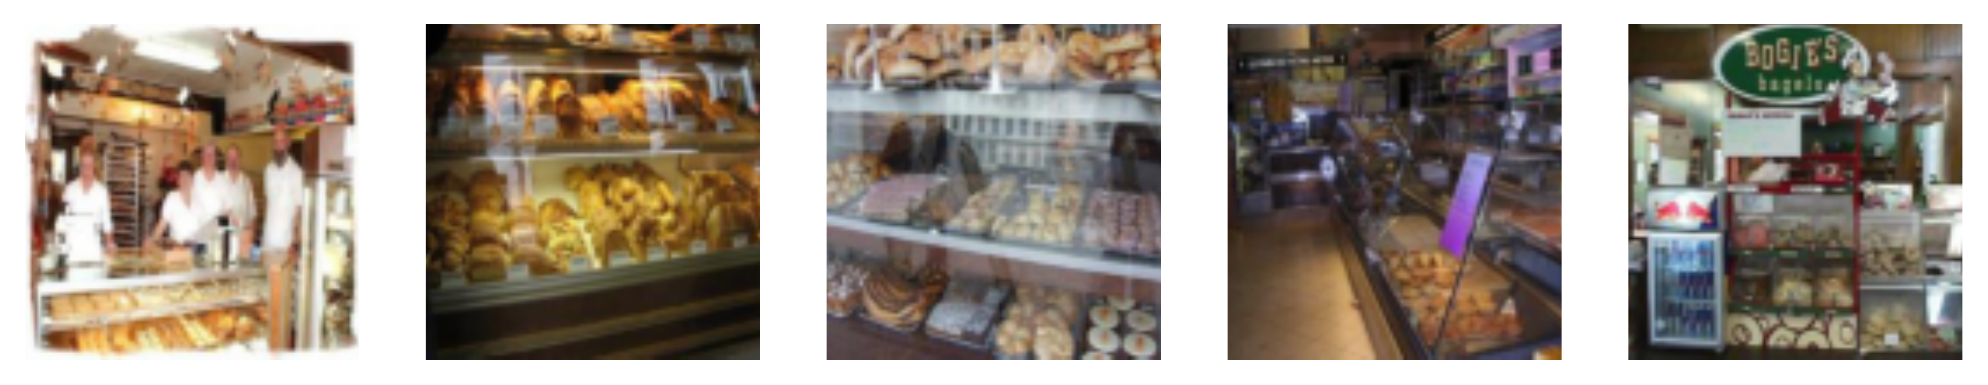}} & \raisebox{-0.4\totalheight}{\includegraphics[width=0.4\textwidth]{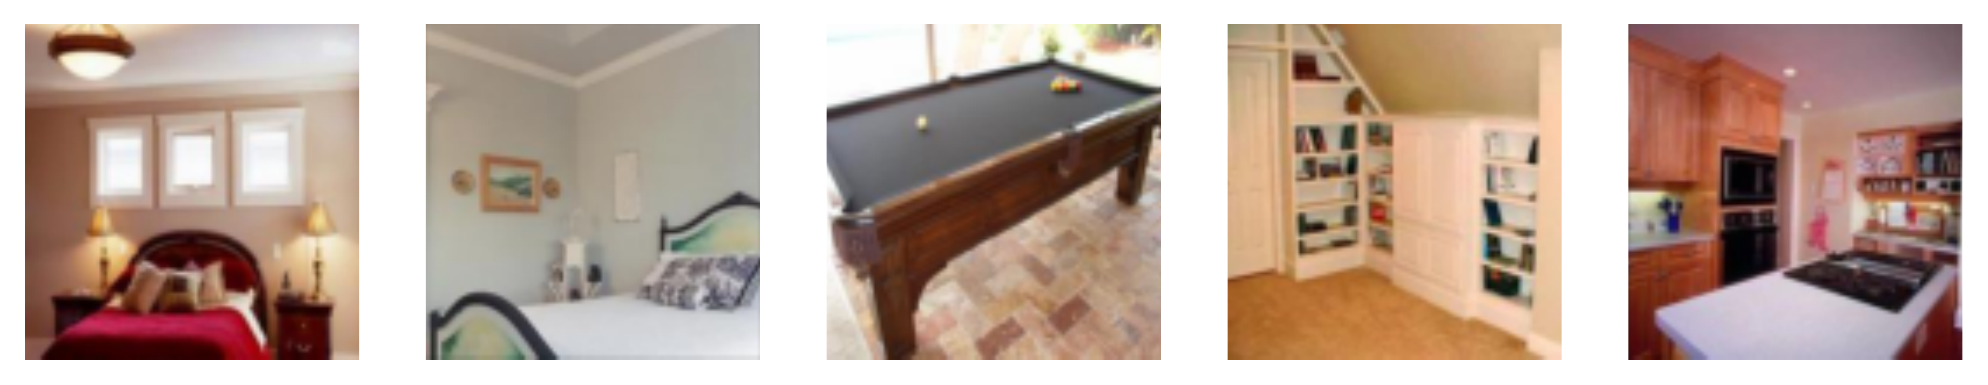}} \\ 
sf, su & \raisebox{-0.4\totalheight}{\includegraphics[width=0.4\textwidth]{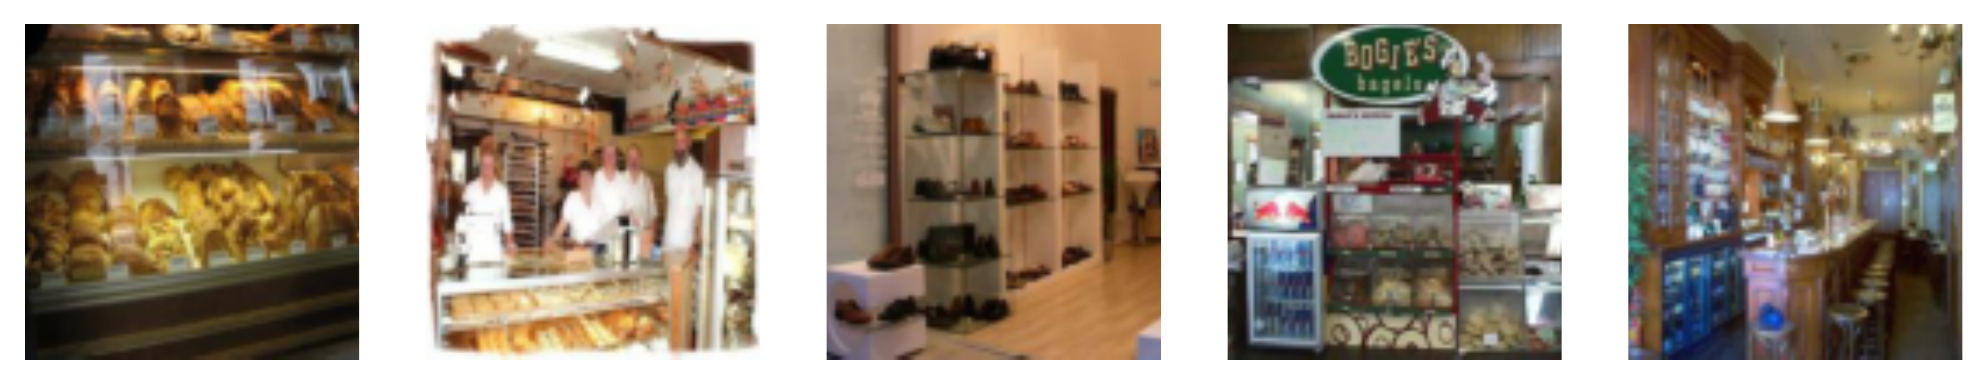}} & \raisebox{-0.4\totalheight}{\includegraphics[width=0.4\textwidth]{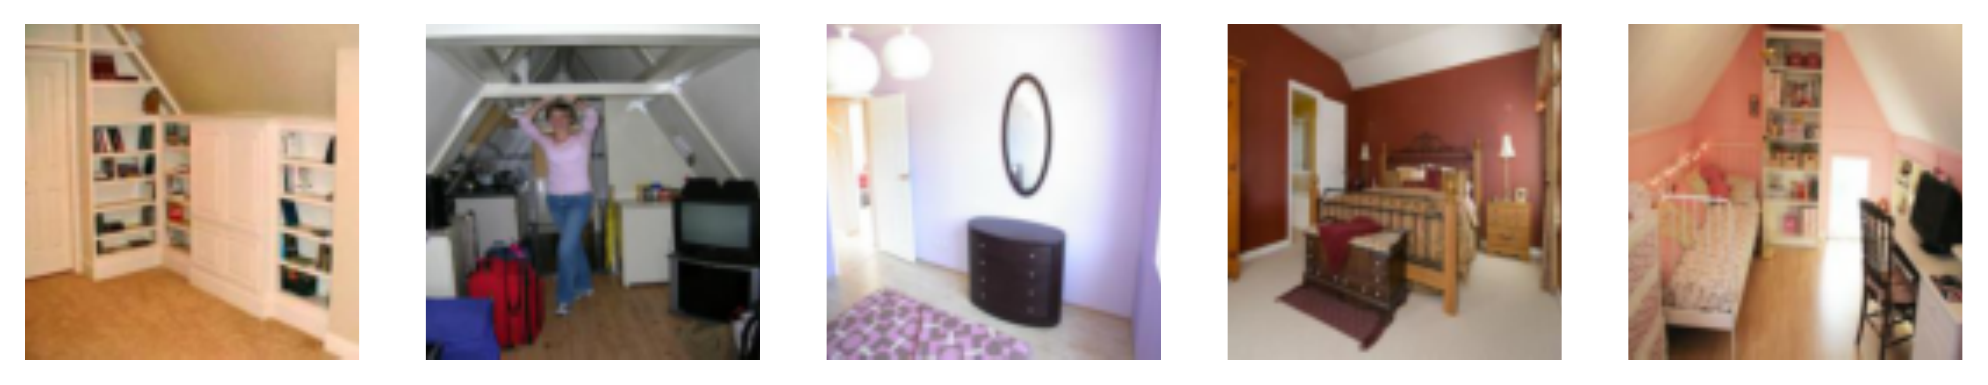}} \\ 
sf, lu & \raisebox{-0.4\totalheight}{\includegraphics[width=0.4\textwidth]{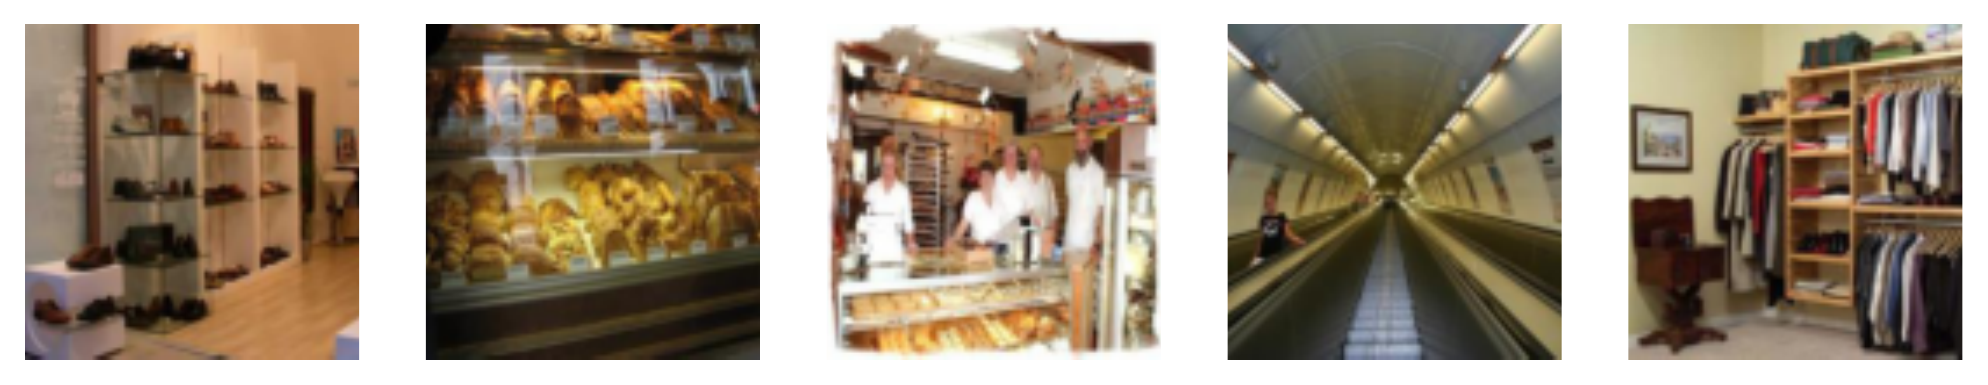}} & \raisebox{-0.4\totalheight}{\includegraphics[width=0.4\textwidth]{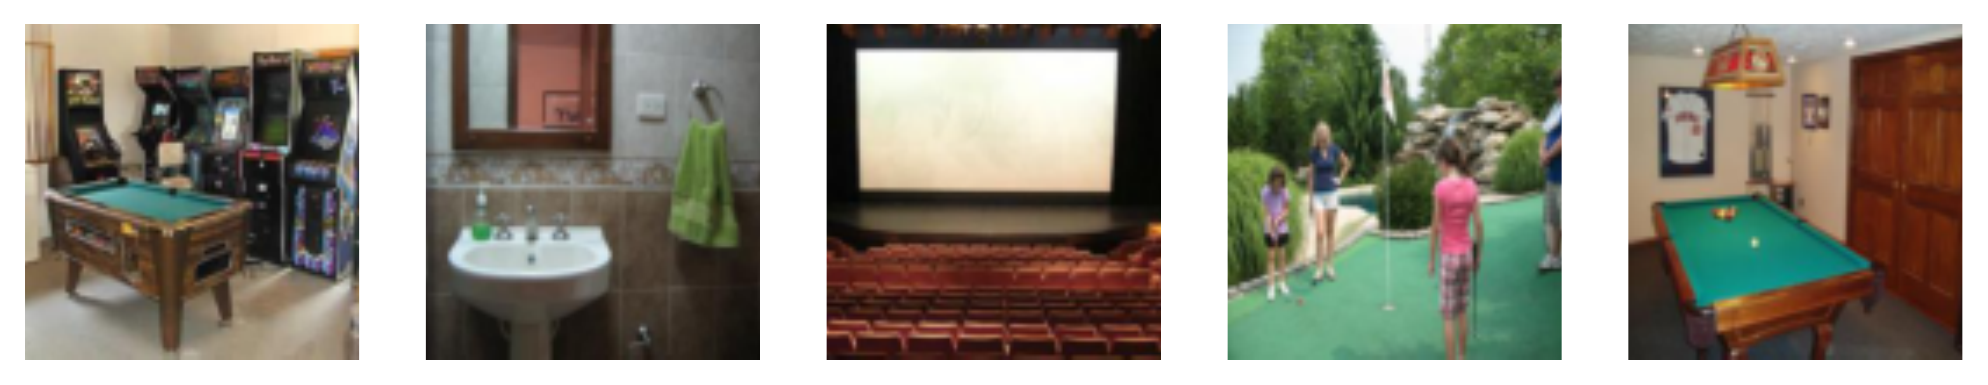}} \\ 
\midrule
& workplace (machines?) &  industrial/construction (smoke stack, garbage?) \\\midrule
sf, mu & \raisebox{-0.4\totalheight}{\includegraphics[width=0.4\textwidth]{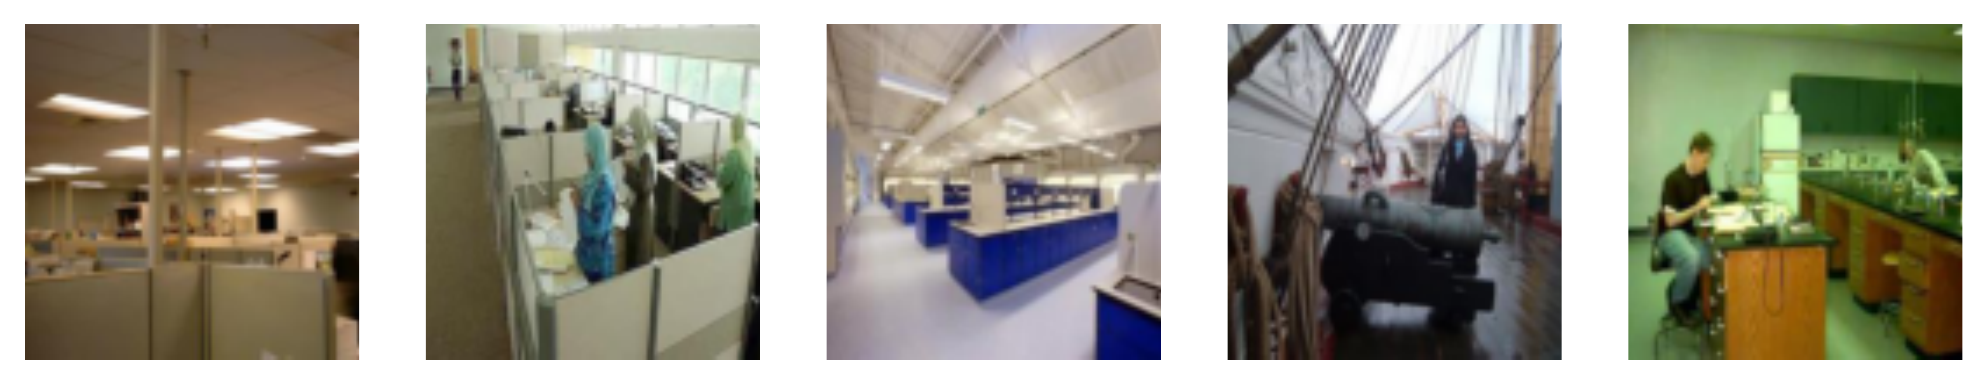}} & \raisebox{-0.4\totalheight}{\includegraphics[width=0.4\textwidth]{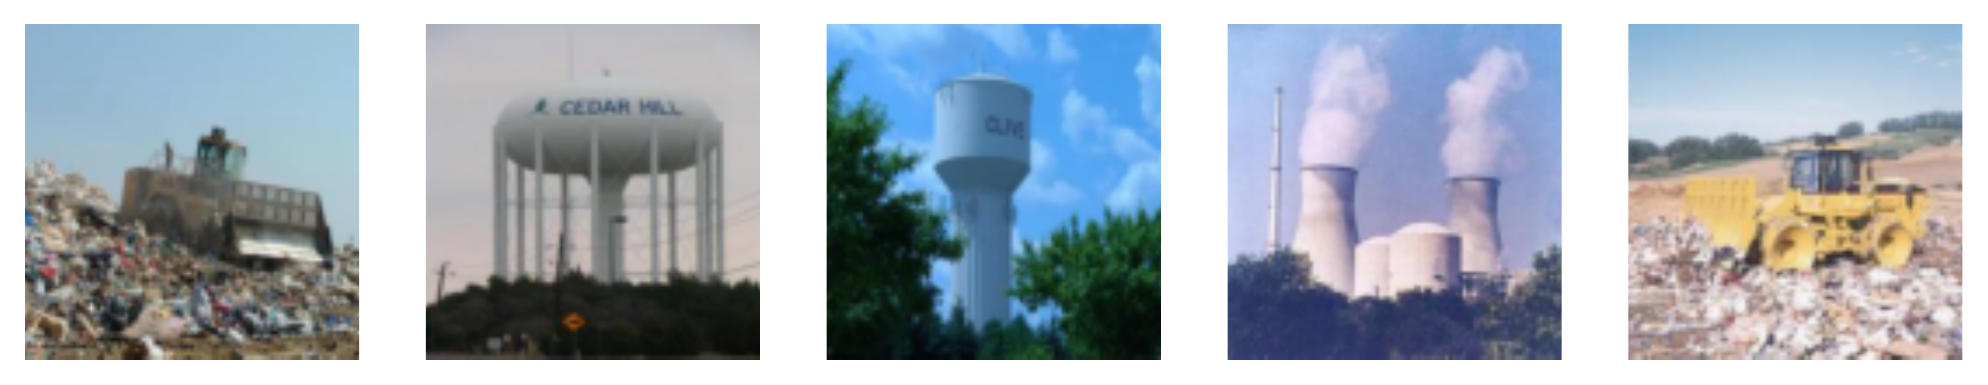}} \\ 
sf, su & \raisebox{-0.4\totalheight}{\includegraphics[width=0.4\textwidth]{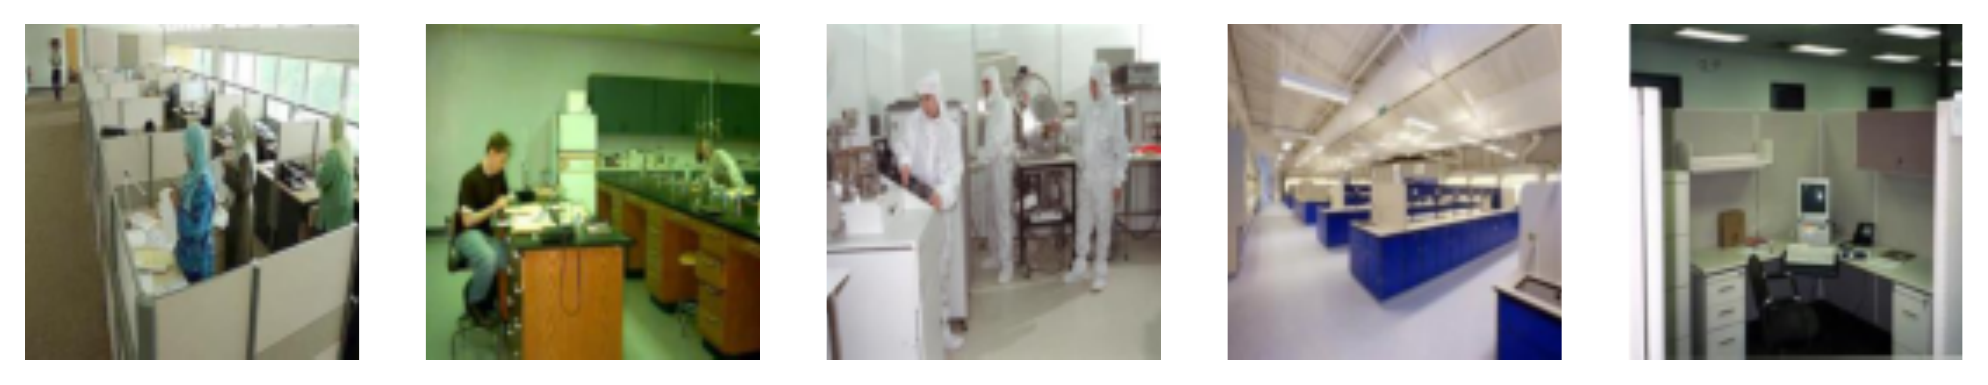}} & \raisebox{-0.4\totalheight}{\includegraphics[width=0.4\textwidth]{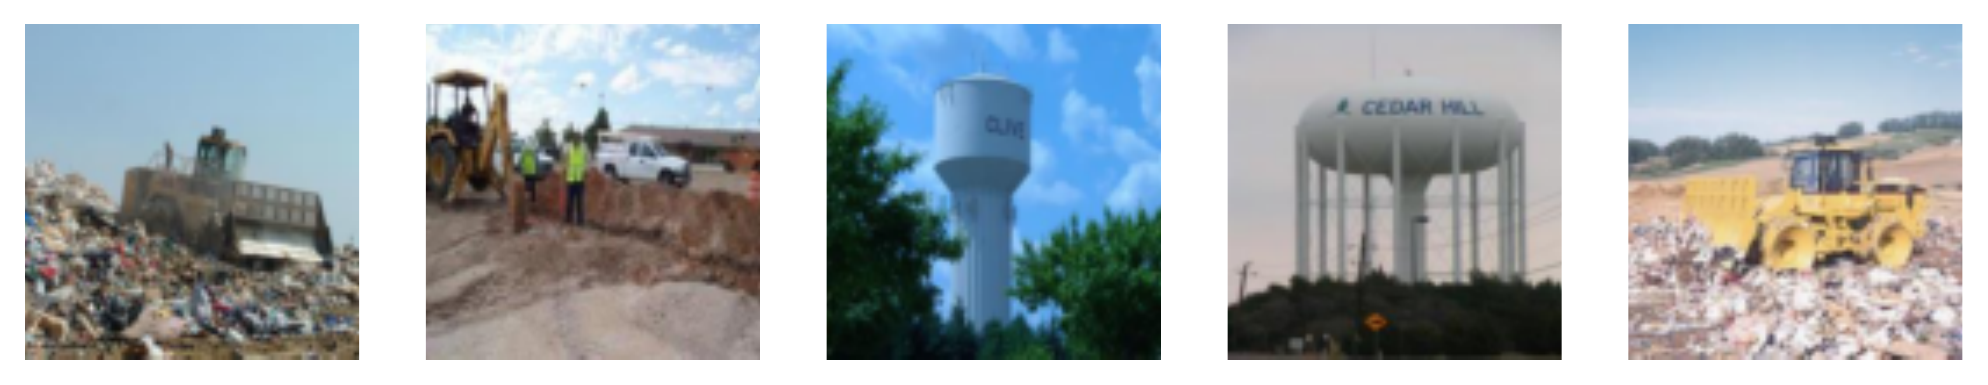}} \\ 
sf, lu & \raisebox{-0.4\totalheight}{\includegraphics[width=0.4\textwidth]{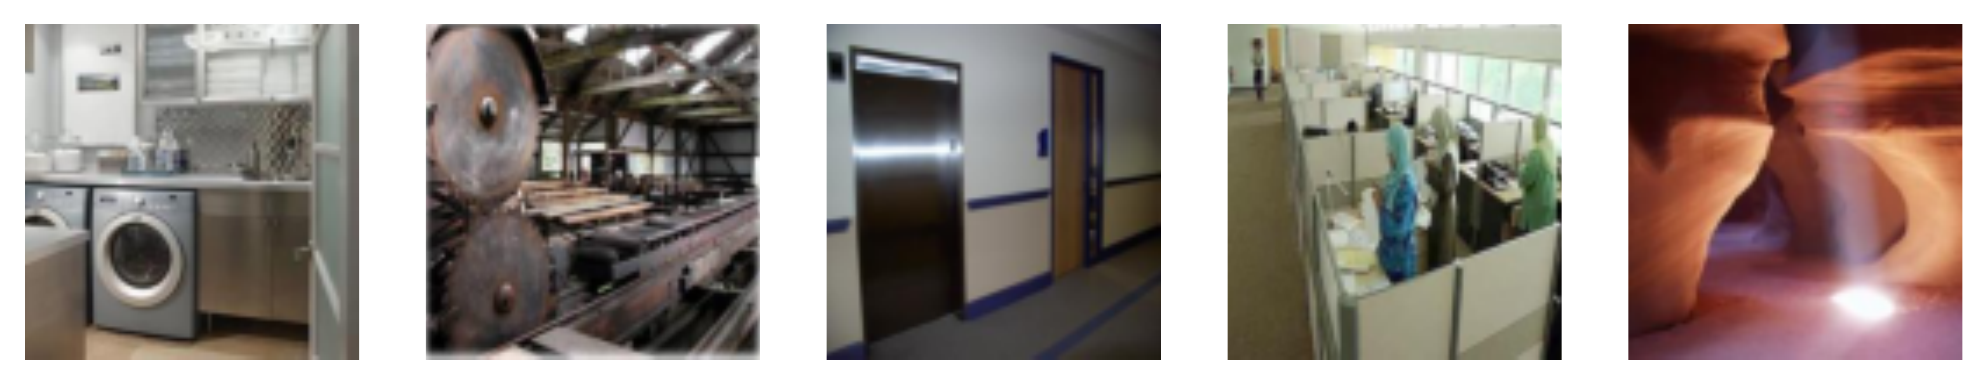}} & \raisebox{-0.4\totalheight}{\includegraphics[width=0.4\textwidth]{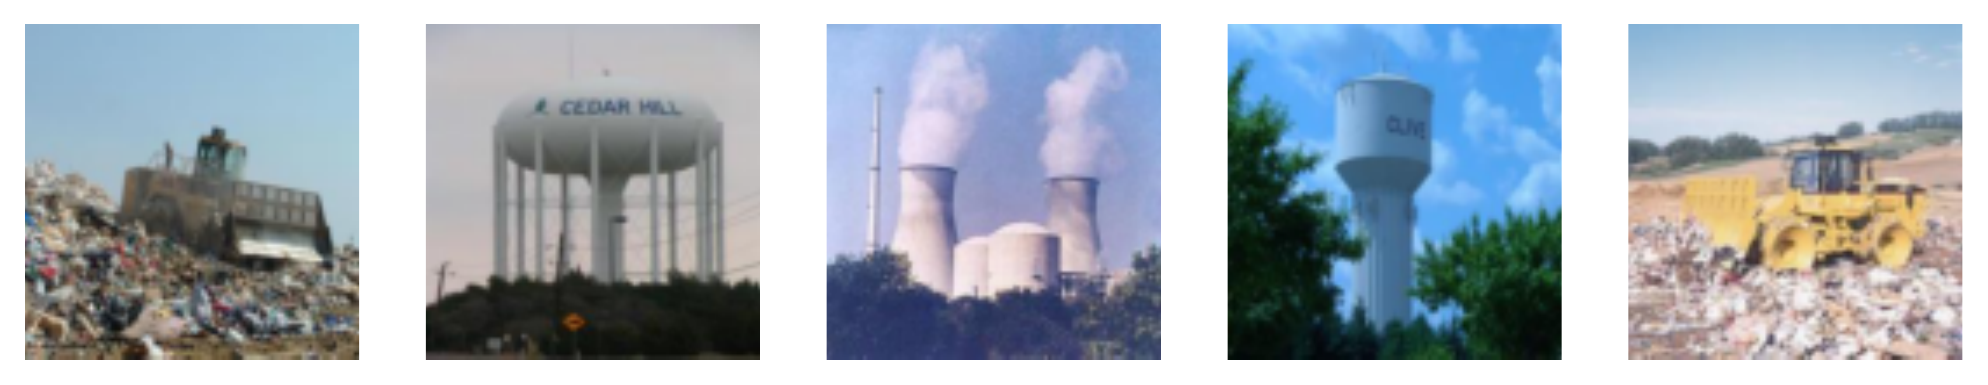}} \\ 
\bottomrule
\end{tabular}
\caption{\textbf{Visualizing the remainder}. We compute  $v = F(x) - h_\text{pred} \circ h_\text{conc}(x)$ and show the top 5 images for which $v_k$ corresponding to these classes is the largest (i.e., the images that are most poorly explained) for more coarse scene groups (similar to Fig. 4 in the main text). For classes that are well explained by the model (e.g. home/hotel), we see that the images no longer correspond to the class. We propose additional concepts for other classes in parenthesis.  }
\label{fig:remainder_group}
\end{figure*}
